# Supplementary material for: DELPHIC: Practical DEL Planning via Possibilities (Extended Version)
Source: arXiv:2307.15451 source file (2023-07-28)
Supplement: Supplementary file 1 [file appendix.tex]

% This is samplepaper.tex, a sample chapter demonstrating the
% LLNCS macro package for Springer Computer Science proceedings;
% Version 2.21 of 2022/01/12
%
\documentclass[runningheads]{llncs}
\usepackage[T1]{fontenc}
% T1 fonts will be used to generate the final print and online PDFs,
% so please use T1 fonts in your manuscript whenever possible.
% Other font encondings may result in incorrect characters.
%
\usepackage{graphicx}
% Used for displaying a sample figure. If possible, figure files should
% be included in EPS format.
%
% If you use the hyperref package, please uncomment the following two lines
% to display URLs in blue roman font according to Springer's eBook style:
%\usepackage{color}
%\renewcommand\UrlFont{\color{blue}\rmfamily}
%

%%% Added packages %%%
\usepackage{amssymb}
\usepackage[english]{babel}
\usepackage[all]{foreign}
\usepackage{multirow}
\usepackage{paralist}
\usepackage[inline]{enumitem} % must be after paralist
\usepackage{subfig}
\usepackage{tikz}

%% Tikz settings %%
\tikzset{every picture/.style={line width=0.75pt}}
\usetikzlibrary{arrows,positioning,calc}

\input{../macros.tex}

\begin{document}
    \title{\textsc{delphic}: Practical DEL Planning via Possibilities (Appendix)}
    
    %\titlerunning{Abbreviated paper title}
    % If the paper title is too long for the running head, you can set
    % an abbreviated paper title here
    
    \author{
        Alessandro Burigana\inst{1}\orcidID{0000-0002-9977-6735} \and
        Paolo Felli\inst{2}\orcidID{0000-0001-9561-8775} \and
        Marco Montali\inst{1}\orcidID{0000-0002-8021-3430}
    }
    
    \authorrunning{A. Burigana et al.}
    % First names are abbreviated in the running head.
    % If there are more than two authors, 'et al.' is used.
    
    \institute{
        Free University of Bozen-Bolzano, Italy
        \email{\{burigana, montali\}@inf.unibz.it}
        \and
        University of Bologna, Italy
        \email{paolo.felli@unibo.it}
    }
    
    \maketitle              % typeset the header of the contribution

    \appendix

    \input{tex/a1_full_proofs.tex}
    \input{tex/a2_asp.tex}
    \input{tex/a3_domains.tex}
    \input{tex/a4_comparison.tex}
    \input{tex/a5_tables.tex}

    %
    % ---- Bibliography ----
    %
    % BibTeX users should specify bibliography style 'splncs04'.
    % References will then be sorted and formatted in the correct style.
    %
    \bibliographystyle{splncs04}
    \bibliography{bibliography}
\end{document}
